# Supplementary material for: A Predictive Chance Constraint Rebalancing Approach to Mobility-on-Demand Services
Source: arXiv:2209.03214 source file (2023-01-15)
Supplement: Supplementary file 1 [file appendices.tex]

\appendices

\section{}

\glsaddall
\printglossary
